# Supplementary material for: Bayesian spatio-temporal model for high-resolution short-term forecasting of precipitation fields
Source: arXiv:2105.03269 ancillary file (2021-05-07)
Supplement: Supplementary file 1 [file supplementary.pdf]

SUPPLEMENTARY MATERIAL FOR

*A Bayesian spatio-temporal model for high-resolution short-term forecasting of precipitation fields*

S. R. Johnson, S. E. Heaps, K. J. Wilson, D. J. Wilkinson

# 1 Discretisation scheme

Here we outline the discretisation of the advection-diffusion-reaction equation (3) in the paper and note that the solution to the diffusion-reaction equation (4) of the source-sink process can be straightforwardly obtained by fixing $v_x^t = v_y^t = 0\ \forall t$ and letting $\theta \to S$, $a \to a^*$, $b \to b^*$, $S + \epsilon \to \tilde{\epsilon}$ in what follows.

The advection-diffusion-reaction equation is given by

$$\frac{\partial \theta}{\partial t} = b\left[\frac{\partial^2 \theta}{\partial x^2} + \frac{\partial^2 \theta}{\partial y^2}\right] - \left[v_x^t \frac{\partial \theta}{\partial x} + v_y^t \frac{\partial \theta}{\partial y}\right] - a\theta + S + \epsilon, \tag{1}$$

and note that we can rewrite this equation as

$$\frac{\partial \theta}{\partial t} = f_0(\theta) + f_1(\theta),$$

where

$$f_0(\theta) = b\left[\frac{\partial^2 \theta}{\partial x^2} + \frac{\partial^2 \theta}{\partial y^2}\right] - \left[v_x^t \frac{\partial \theta}{\partial x} + v_y^t \frac{\partial \theta}{\partial y}\right], \quad \text{and} \quad f_1(\theta) = -a\theta + S + \epsilon.$$

A numerical solution to (1) can then be obtained by sequentially solving the sub-problems

$$\frac{\partial \tilde{\theta}}{\partial t} = f_0(\tilde{\theta}) \quad \text{with inital conditon} \quad \tilde{\theta}^t = \theta^t \tag{2}$$

$$\frac{d\breve{\theta}}{dt} = f_1(\breve{\theta}) \quad \text{with inital conditon} \quad \breve{\theta}^t = \tilde{\theta}^{t+1} \tag{3}$$

and the solution to (1) at time $t+1$ is given by $\theta^{t+1} = \breve{\theta}^{t+1}$.

## 1.1 Sub-problem 1

The first sub-problem given by (2) corresponds to the advection diffusion equation. As outlined in Section 2.1 of the paper we take a FTCS solution and so the partial derivatives are approximated by $\partial\theta/\partial t \simeq (\theta_{ij}^{t+1} - \theta_{ij}^t)/\delta t$, $\partial\theta/\partial x \simeq (\theta_{i+1,j}^t - \theta_{i-1,j}^t)/2\delta x$, $\partial\theta/\partial y \simeq (\theta_{i,j+1}^t - \theta_{i,j-1}^t)/2\delta y$, $\partial^2\theta/\partial x^2 \simeq (\theta_{i+1,j}^t + \theta_{i-1,j}^t - 2\theta_{ij}^t)/(\delta x)^2$ and $\partial^2\theta/\partial y^2 \simeq (\theta_{i,j+1}^t + \theta_{i,j+1}^t - 2\theta_{ij}^t)/(\delta y)^2$. Note that here we consider a regular lattice grid

and so we let $\delta d \equiv \delta x = \delta y$. Using the approximations above with $\delta t = 1$ and recalling that $\tilde{\theta}^t = \theta^t$ yields the following.

$$
\begin{aligned}
& \frac{\partial \tilde{\theta}}{\partial t} = f_0(\tilde{\theta}) \\
\implies \quad & \frac{\partial \tilde{\theta}}{\partial t} = b\left[\frac{\partial^2\theta}{\partial x^2} + \frac{\partial^2\theta}{\partial y^2}\right] - \left[v_x^t\frac{\partial\theta}{\partial x} + v_y^t\frac{\partial\theta}{\partial y}\right] \\
\implies \quad & \tilde{\theta}_{ij}^{t+1} - \theta_{ij}^t = \frac{b}{(\delta d)^2}\left[\theta_{i+1,j}^t + \theta_{i-1,j}^t - 2\theta_{ij}^t + \theta_{i,j+1}^t + \theta_{i,j+1}^t - 2\theta_{ij}^t\right] \\
& \qquad - \left[\frac{v_x^t}{2\delta d}(\theta_{i+1,j}^t - \theta_{i-1,j}^t) + \frac{v_y^t}{2\delta d}(\theta_{i,j+1}^t - \theta_{i,j-1}^t)\right] \\
\implies \quad & \tilde{\theta}_{ij}^{t+1} = \left(1 - \frac{4b}{(\delta d)^2}\right)\theta_{ij}^t + \left(\frac{b}{(\delta d)^2} + \frac{v_x^t}{2\delta d}\right)\theta_{i-1,j}^t + \left(\frac{b}{(\delta d)^2} - \frac{v_x^t}{2\delta d}\right)\theta_{i+1,j}^t \\
& \qquad + \left(\frac{b}{(\delta d)^2} + \frac{v_y^t}{2\delta d}\right)\theta_{i,j-1}^t + \left(\frac{b}{(\delta d)^2} - \frac{v_y^t}{2\delta d}\right)\theta_{i,j+1}^t
\end{aligned}
$$

and letting $\beta = b/(\delta d)^2$, $\nu_x^t = v_x^t/2\delta d$ and $\nu_y^t = v_y^t/2\delta d$ gives

$$
\begin{aligned}
\tilde{\theta}_{ij}^{t+1} = (1-4\beta)\theta_{ij}^t &+ \left(\beta + \nu_x^t\right)\theta_{i-1,j}^t + \left(\beta - \nu_x^t\right)\theta_{i+1,j}^t \\
&+ \left(\beta + \nu_y^t\right)\theta_{i,j-1}^t + \left(\beta - \nu_y^t\right)\theta_{i,j+1}^t.
\end{aligned}
$$

## 1.2 Sub-problem 2

Sub-problem 2 is given by (3) and corresponds to a simple decay function with additive forcing terms. As outlined in Section 2.1 of the paper we take a first-order forward time solution and so the derivative is approximated by $d\theta/dt \simeq (\theta_{ij}^{t+1} - \theta_{ij}^t)/\delta t$. Initialising this equation with the solution to sub-problem 1, that is, letting $\breve{\theta}^t = \tilde{\theta}^{t+1}$ gives

$$
\begin{aligned}
& \frac{d\breve{\theta}}{dt} = f_1(\breve{\theta}) \\
\implies \quad & \frac{\partial \breve{\theta}}{\partial t} = -a\breve{\theta} + S + \epsilon \\
\implies \quad & \breve{\theta}_{ij}^{t+1} - \tilde{\theta}_{ij}^{t+1} = -a\tilde{\theta}_{ij}^{t+1} + S_{ij}^t + \epsilon_{ij}^t \\
\implies \quad & \breve{\theta}_{ij}^{t+1} = (1-a)\tilde{\theta}_{ij}^{t+1} + S_{ij}^t + \epsilon_{ij}^t
\end{aligned}
$$

and letting $\alpha = (1-a)$ allows us to write

$$
\breve{\theta}_{ij}^{t+1} = \alpha\tilde{\theta}_{ij}^{t+1} + S_{ij}^t + \epsilon_{ij}^t.
$$

### 1.3 Combing solutions

The solution to (1) can now be obtained by combining the solution to the two sub-problems outlined in the previous two subsections. In particular the solution is $\theta^{t+1} = \breve{\theta}^{t+1}$ and so

$$\begin{aligned}\theta^{t+1} &= \breve{\theta}^{t+1} \\ &= \alpha\tilde{\theta}_{ij}^{t+1} + S_{ij}^{t} + \epsilon_{ij}^{t} \\ &= \alpha\left[(1-4\beta)\theta_{ij}^{t} + \left(\beta+\nu_x^t\right)\theta_{i-1,j}^{t} + \left(\beta-\nu_x^t\right)\theta_{i+1,j}^{t} + \left(\beta+\nu_y^t\right)\theta_{i,j-1}^{t} + \left(\beta-\nu_y^t\right)\theta_{i,j+1}^{t}\right] \\ &\qquad + S_{ij}^{t} + \epsilon_{ij}^{t},\end{aligned}$$

where $\alpha = (1-a)$, $\beta = b/(\delta d)^2$, $\nu_x^t = v_x^t/2\delta d$ and $\nu_y^t = v_y^t/2\delta d$.

As noted in Section 1 the solution to the diffusion-reaction equation, that is, equation (4) in the paper, can be straightforwardly obtained by fixing $v_x^t = v_y^t = 0\ \forall t$ and letting $\theta \to S$, $a \to a^*$, $b \to b^*$, $S + \epsilon \to \tilde{\epsilon}$ and so

$$S^{t+1} = \alpha^*\left[(1-4\beta^*)S_{ij}^{t} + \beta^* S_{i-1,j}^{t} + \beta^* S_{i+1,j}^{t} + \beta^* S_{i,j-1}^{t} + \beta^* S_{i,j+1}^{t}\right] + \tilde{\epsilon}_{ij}^{t},$$

where $\alpha^* = (1-a^*)$ and $\beta^* = b^*/(\delta d)^2$.

## 2 Covariance estimation

Key to the successful implementation of the EnKS algorithm is the effective estimation of the (cross-)covariance matrices required to construct the approximate Kalman gain matrix $\hat{K}_{\ell t}$. The matrices to be approximated from the ensemble are $\Sigma_{\ell t|t-1}^{xy}$ and $\Sigma_{tt|t-1}^{yy}$. These matrices are of dimension $N^{\mathrm{s}} \times N^{\mathrm{o}}$ and $N^{\mathrm{o}} \times N^{\mathrm{o}}$ respectively, where $N^{\mathrm{s}} = 2N$ and $N^{\mathrm{o}} = N + N^{\mathrm{g}}$ are the dimension of the state and observation vectors. If $N^{\mathrm{o}}$ is small then it is sensible to approximate both $\Sigma_{\ell t|t-1}^{xy}$ and $\Sigma_{tt|t-1}^{yy}$ directly from the ensembles $\mathcal{X}_{\ell|t-1}$ and $\mathcal{Y}_{t|t-1}$ as described in Section 5.3 of the paper; where reasonable approximations are likely to be obtained with $N^{\mathrm{e}} \gg N^{\mathrm{o}}$. Alternatively, if $N^{\mathrm{s}}$ is small then we can approximate these matrices based solely on the state ensemble as $\Sigma_{\ell t|t-1}^{xy} \doteq \Sigma_{\ell t|t-1}F'$ and $\Sigma_{tt|t-1}^{yy} \doteq F\Sigma_{tt|t-1}F' + V$, where $\Sigma_{\ell t|t-1}$ is the (cross-)covariance of the state ensembles $\mathcal{X}_{\ell|t-1} = (\boldsymbol{x}_{\ell|t-1}^{1}, \ldots, \boldsymbol{x}_{\ell|t-1}^{N^{\mathrm{e}}})$ and $\mathcal{X}_{t|t-1} = (\boldsymbol{x}_{t|t-1}^{1}, \ldots, \boldsymbol{x}_{t|t-1}^{N^{\mathrm{e}}})$. Note that $\doteq$ denotes the equivalence only holds in the asymptotic limit of infinite ensemble size. Again, reasonable approximations are likely to be obtained when $N^{\mathrm{e}} \gg N^{\mathrm{s}}$.

That said, as in our application, the EnKS approximation is typically used in settings where both the state and observation dimensions are large. In these settings the EnKS algorithm is only computationally feasible for a modest number of ensemble members (typically $N^{\mathrm{e}} \leq 100$) and so in general $N^{\mathrm{e}} \ll N^{\mathrm{s}}, N^{\mathrm{o}}$ and care

must be taken when estimating the (cross-)covariance matrices. Several methods have been proposed for improving the accuracy of the covariance approximations in this setting, most commonly, *covariance tapering* (Houtekamer and Mitchell, 2001) and *covariance inflation* (Anderson and Anderson, 1999) however there is little guidance on how to choose an appropriate tapering function and/or inflation factor. The approach we favour, and also that which we find works well in practice, relies on approximating the matrices from the so-called *deterministic ensemble* and then using analytic results to obtain the required matrix. This is particularly appealing as, not only does it not require an ad-hoc choice of tapering function and/or inflation parameter, it also preserves the asymptotic result that exact samples are obtained in the limit of $N^{\mathrm{e}} \to \infty$. To implement this approach we introduce $\tilde{\boldsymbol{x}}^j_{t|t-1} = \tilde{G}_t \boldsymbol{x}^j_{t-1|t-1}$ in Step 1 of the EnKS algorithm and let $\boldsymbol{x}^j_{t|t-1} = \tilde{\boldsymbol{x}}^j_{t|t-1} + \boldsymbol{w}^j_t$ for $j = 1, \ldots, N^{\mathrm{e}}$. The required covariance matrix $\Sigma_{tt|t-1} \doteq \tilde{\Sigma}_{tt|t-1} + W$ where $\tilde{\Sigma}_{tt|t-1}$ is the sample covariance computed from the deterministic ensemble $\tilde{\mathcal{X}}_{t|t-1} = (\tilde{\boldsymbol{x}}^1_{t|t-1}, \ldots, \tilde{\boldsymbol{x}}^{N^{\mathrm{e}}}_{t|t-1})$. Similarly the cross-covariance matrix $\tilde{\Sigma}_{\ell t|t-1}$ is computed from the ensembles $\mathcal{X}_{\ell|t-1}$ and $\tilde{\mathcal{X}}_{t|t-1}$. It follows that the Kalman gain matrix can be written as

$$\hat{K}_{\ell t} = \begin{cases} \tilde{\Sigma}_{\ell t|t-1} F' \left( F \tilde{\Sigma}_{tt|t-1} F' + F W F' + V \right)^{-1}, & \text{for } \ell < t, \\ (\tilde{\Sigma}_{tt|t-1} + W) F'_t \left( F \tilde{\Sigma}_{tt|t-1} F' + F W F' + V \right)^{-1}, & \text{for } \ell = t. \end{cases} \tag{4}$$

The advantage of approximating the matrices in this way is that any spurious correlations between the realisations of the state and observation errors $\boldsymbol{w}^j \sim \mathrm{N}(0, W)$, $\boldsymbol{v}^j \sim \mathrm{N}(0, V)$ do not impact the matrix estimation. Note that $Q_t = \left( F \tilde{\Sigma}_{tt|t-1} F' + F W F' + V \right)$ is an (assumed large) $N^{\mathrm{o}} \times N^{\mathrm{o}}$ matrix and the inverse can be obtained by appealing to the Sherman-Morrison-Woodbury formula; further guidance on the practical implementation of these algorithms is given by Evensen (2003).

# 3 Simulation studies

To investigate the effectiveness of the posterior sampling scheme outlined in Section 5.4 of the paper we consider a synthetic dataset for which the values of the underlying parameters are known. We consider an $N = 72 \times 72$ grid and $N^{\mathrm{g}} = 15$ rain gauges where the gauge locations are sampled uniformly at random. Given values of the static parameters we initialise $\boldsymbol{x}_0$ and $\boldsymbol{\nu}_0$ from the prior distribution and obtain a realisation of the process by drawing from the forward model (12) for $t = 1, \ldots, 656$; the first 300 time points allow the process to converge to its equilibrium distribution and hence are discarded. We then subset the remaining $\tilde{T} = 356$ time points by taking every 5th time point giving rise to $T = 72$ observation times; these data are reproduced within the GitHub repository.

We consider two analyses with the number of imputed time-steps fixed at $\tilde{t} = 4$. In Analysis 1 we implement

a fixed lag smoother in which the states up to and including the previous 3 observation times are smoothed and so $\tau = 3(\tilde{t}+1)$ in the EnKS step (Section 5.3 of the paper); Analysis 2 considers a larger smoothing window with $\tau = 6(\tilde{t}+1)$. The ensemble size is taken to be $N^{\mathrm{e}} = 100$. We initalise the unknown quantities from the prior distribution outlined in Section 4.1 of the paper, more specifically $\boldsymbol{\theta}_0|\mu \sim \mathrm{N}_N(\mu\mathbf{1}_N, 2^2\mathbb{I}_{N\times N})$, $\boldsymbol{S}_0 \sim \mathrm{N}_N(\mathbf{0}, 0.5^2\mathbb{I}_{N\times N})$, $\boldsymbol{\nu}_0 \sim \mathrm{N}_2(\mathbf{0}, 0.1^2\mathbb{I}_2)$, $\mu, \mu_r \sim \mathrm{N}(0,1)$, $\alpha \sim \mathrm{TN}(0.8, 250^{-1}, 0, 1)$ , $\beta \sim \mathrm{N}(0.1, 500^{-1})$ and perform 2000 iterations with the first 1000 discarded as burn-in.

Figure 1 shows boxplots of the marginal posterior distribution of the unknown static parameters $\alpha, \beta, \mu$ and $\mu_r$ for both Analyses 1 and 2; the crosses ($\times$) highlight the value(s) from which these data were simulated and the triangle ($\Delta$) denotes the (marginal) posterior mean(s). From Figure 1 (right) we see that both $\mu$ and $\mu_r$ are well recovered in each case, that is, there is reasonable posterior support for the synthetic values used to generate these data. The auto-regressive parameter $\alpha$ is also fairly well recovered, although, perhaps unsurprisingly, the synthetic value has larger support under Analysis 2 that considers a larger the smoothing window. Interestingly both analyses struggle to recover the synthetic value of $\beta = 0.18$ with $\mathrm{E}(\beta|\mathcal{D}) = 0.213, 0.212$ for Analysis 1 and 2, respectively. That said, it is pleasing to see that the velocity components $\boldsymbol{\nu}_t$ are generally well recovered with the majority of the synthetic values looking plausible under their marginal posterior distributions for both analyses; Figure 2 shows the marginal posterior means, the 95% credible regions, and also the values of the velocity components $\nu_x$ (top) and $\nu_y$ (bottom) from which these data were simulated for both Analysis 1 and 2, left and right, respectively.

The result of reducing the smoothing window within the EnKS step is perhaps most likely to manifest itself within the inferences for the latent process $\boldsymbol{x}_t$. Figure 3 shows image plots of $\mathrm{E}(\theta_{ti}|\mathcal{D})$, that is, the marginal

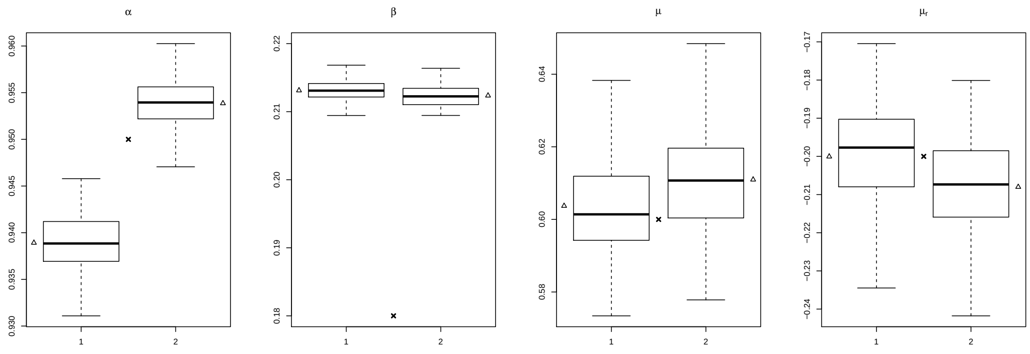


Figure 1: Boxplots of the marginal posterior distribution of the unknown static parameters for analyses 1 and 2; crosses ($\times$) highlight the value from which these data were simulated, triangle ($\Delta$) denotes the posterior mean.

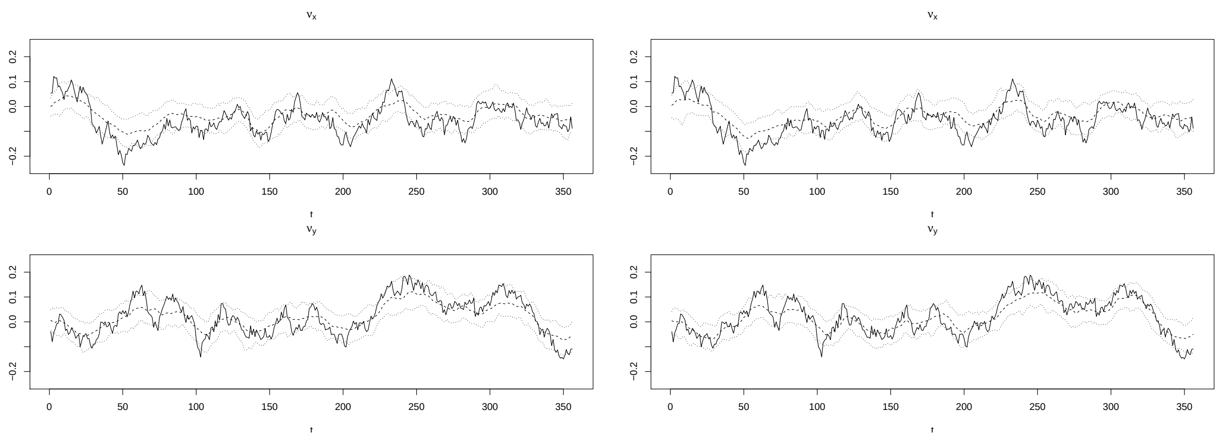


Figure 2: Marginal posterior means (- -), $95\%$ credible regions ($\cdots$), and the synthetic values (–) for the velocity components $\nu_x$ (top) and $\nu_y$ (bottom) under Analysis 1 (left) and Analysis 2 (right) for $t = 1, \ldots, \tilde{T}$.

posterior means of the latent process of interest ($\theta$) for all locations ($i = 1, \ldots, n$) and 6 equally spaced observation time points ($t \in \{12, 24, 36, 48, 60, 72\}$); the corresponding plots for all time-steps are shown in Section 3.1. A visual comparison of the results from Analysis 1 (top) with those from Analysis 2 (middle) suggests that reducing the smoothing window from 6 to 3 has little impact on the state inference. In particular similar spatial clusters of positive (and negative) surface water rates are recovered under both analyses. The bottom row of Figure 3 shows the absolute value of the difference between the inferred means which again highlights how reducing the smoothing window has negligible impact on the state inference.

Turning now to inference for observable quantities, Figure 4 shows the posterior predictive distribution for the gauge (left) and radar (right) observations at a typical gauge location (grid location 1203) for Analysis 1 and 2, top and bottom, respectively. Figures 5 and 6 show the equivalent plots for two additional gauge sites, grid locations 2993 and 4512, respectively. It is pleasing to see that the observed data look like a plausible realisation from the predictive distribution and there is no notable differences between the two analyses; this is perhaps not surprising given that inferences for $\theta$ are similar under each analysis. Thus, based on these synthetic analyses, we suggest that a smoothing widow of $\tau = 3(\tilde{t} + 1)$ is sufficient to obtain reasonable inferences about the quantities of interest.

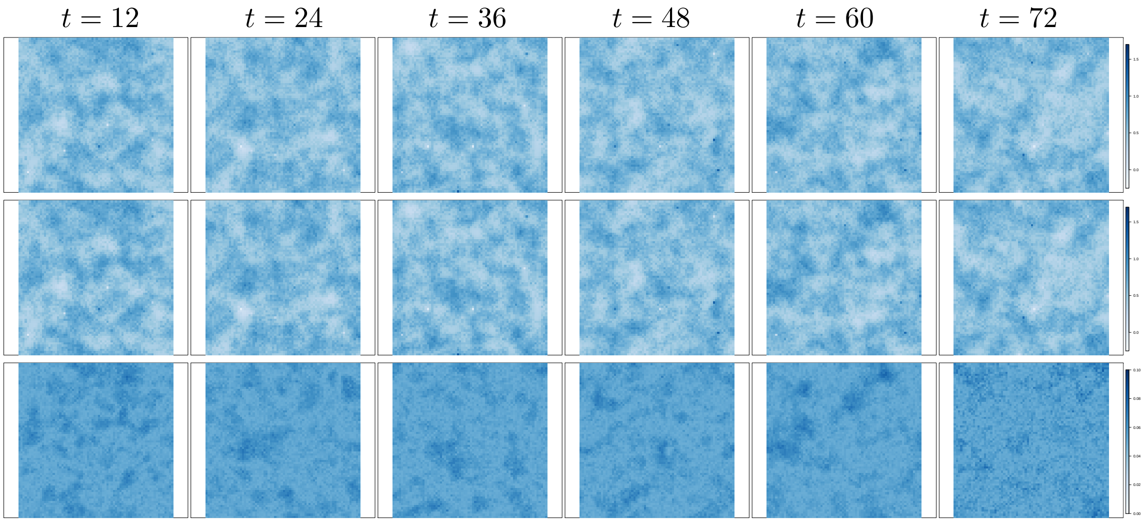


Figure 3: Marginal posterior means of the latent process $\mathrm{E}(\theta_{ti}|\mathcal{D})$ obtained under Analysis 1 (top) and Analysis 2 (middle) and also the absolute value of the difference between the inferred means (bottom).

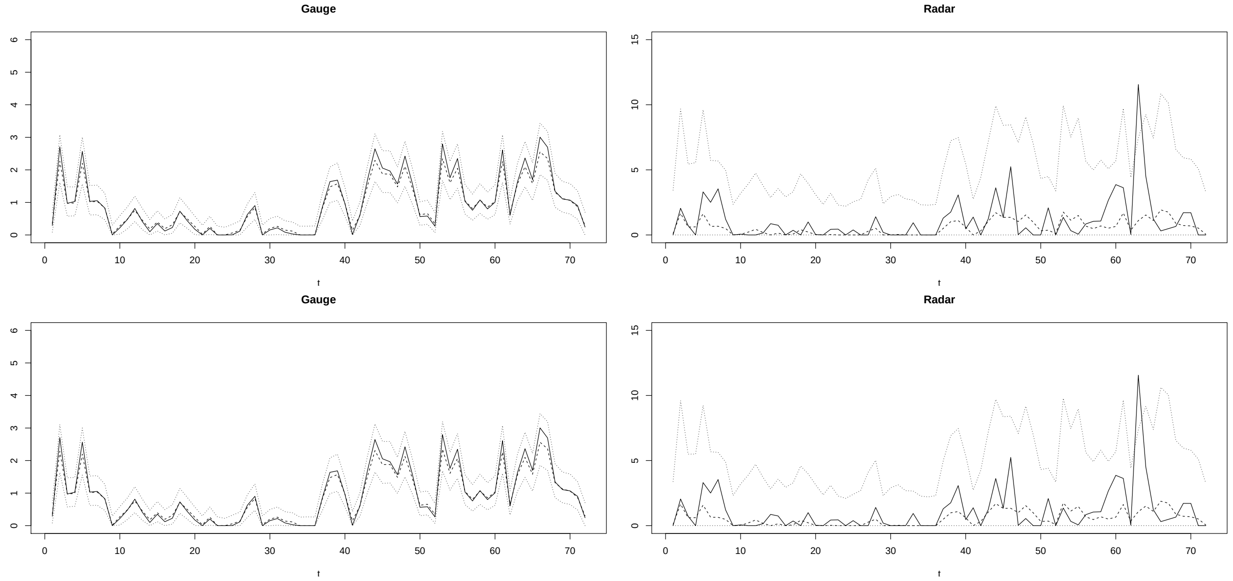


Figure 4: Posterior predictive mean (- -), 95% credible regions ($\cdots$) together with the (synthetic) gauge (left) and radar (right) observations (–) at grid location 1203 for Analysis 1 and 2, top and bottom, respectively.

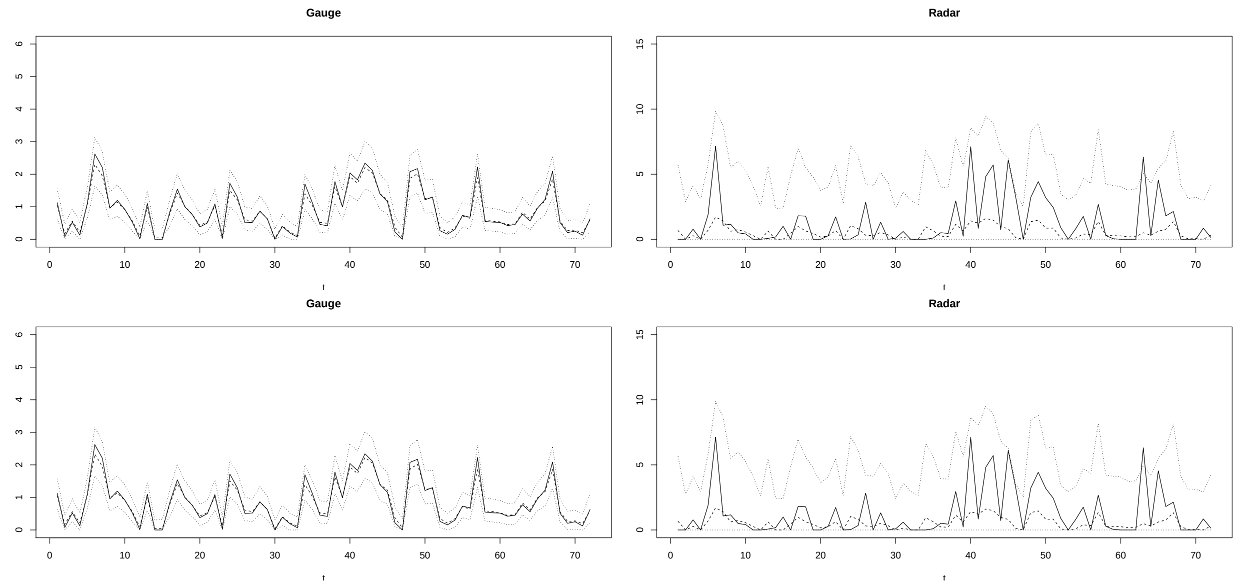


Figure 5: Posterior predictive mean (- -), $95\%$ credible regions $(\cdots)$ together with the (synthetic) gauge (left) and radar (right) observations (–) at grid location $2993$ for Analysis 1 and 2, top and bottom, respectively.

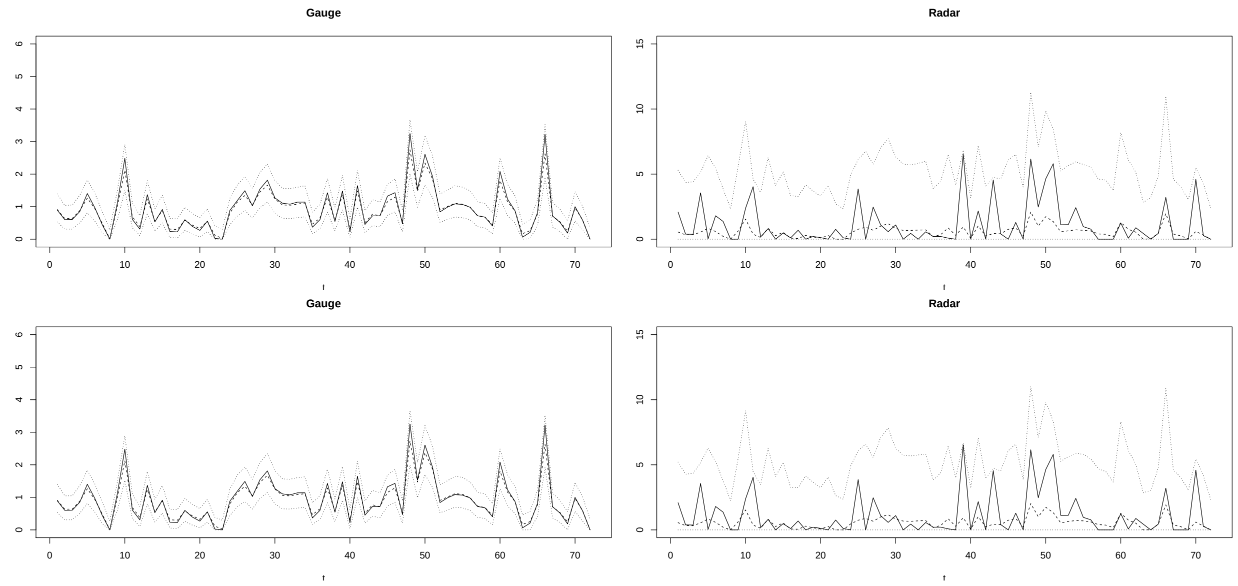


Figure 6: Posterior predictive mean (- -), $95\%$ credible regions $(\cdots)$ together with the (synthetic) gauge (left) and radar (right) observations (–) at grid location $4512$ for Analysis 1 and 2, top and bottom, respectively.

## 3.1 Image plots of the marginal posterior means of the latent process $\theta$

This section contains figures akin to Figure 3 for all observation times $t = 1, \ldots, 72$. That is, each collection of image plots shows the marginal posterior means of the latent process $\mathrm{E}(\theta_{ti}|\mathcal{D})$ obtained under Analysis 1 (top) and Analysis 2 (middle) and also the absolute value of the difference between the inferred means (bottom).

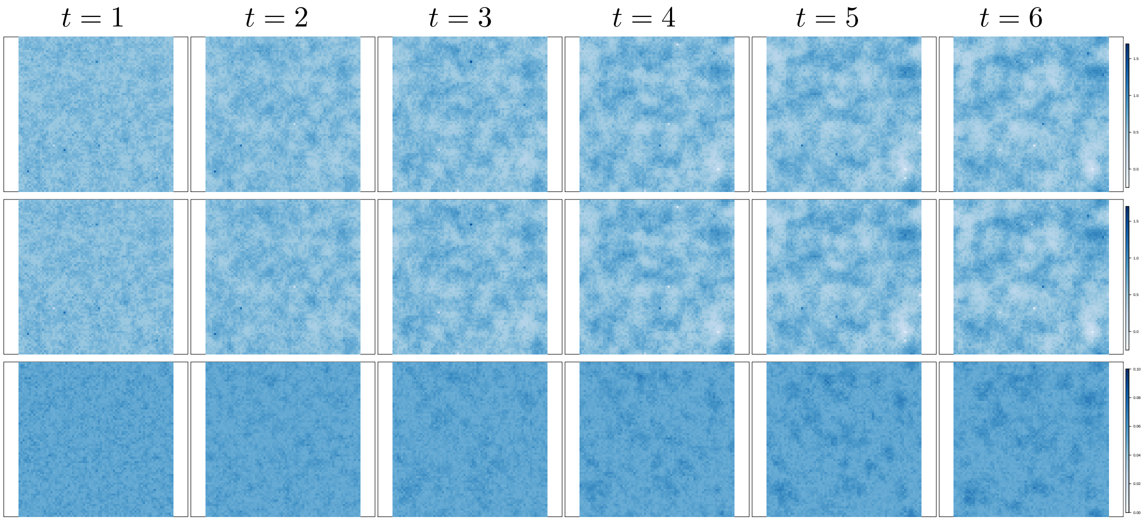


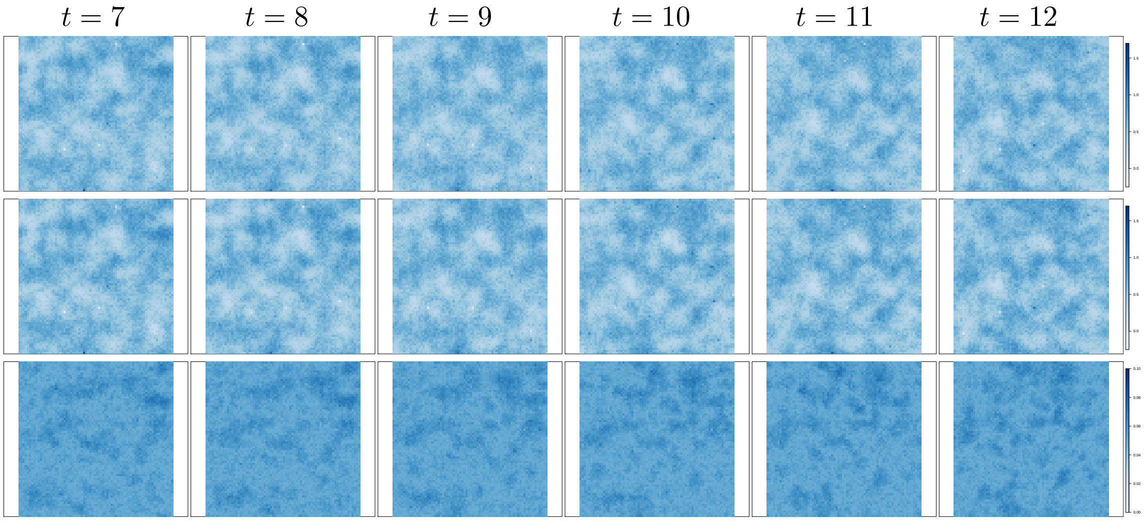

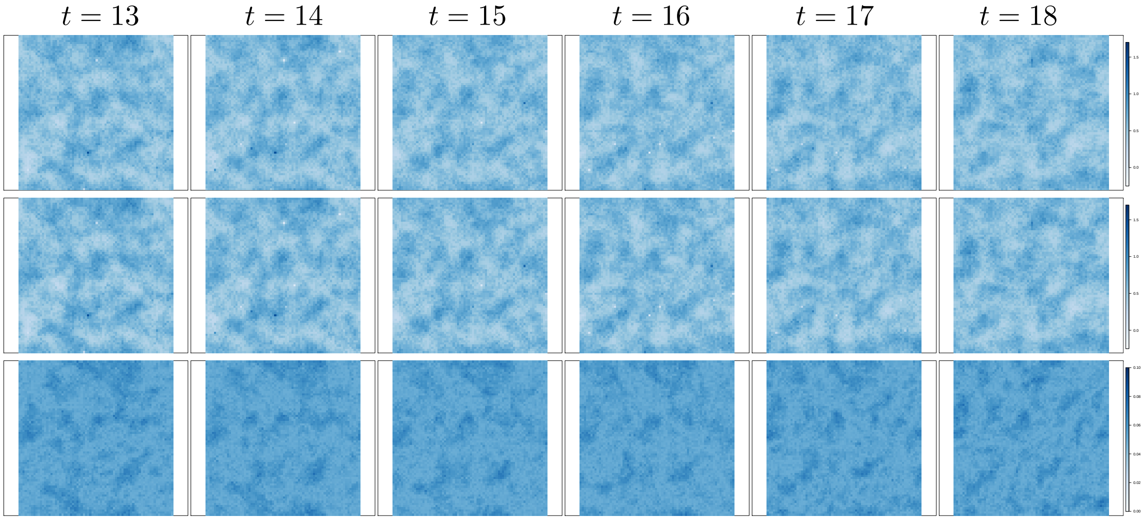
$t = 13$
$t = 14$
$t = 15$
$t = 16$
$t = 17$
$t = 18$

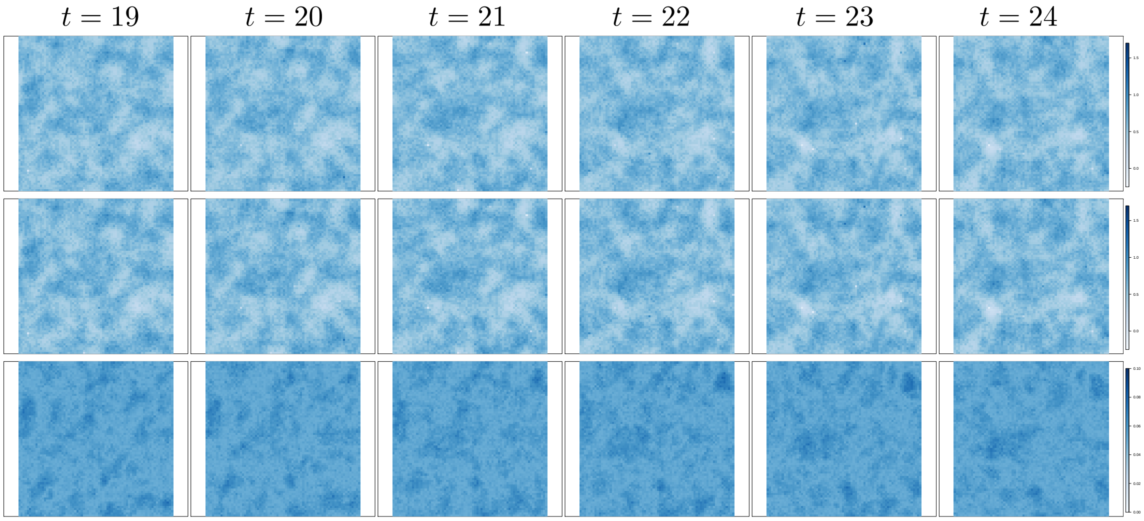
$t = 19$
$t = 20$
$t = 21$
$t = 22$
$t = 23$
$t = 24$

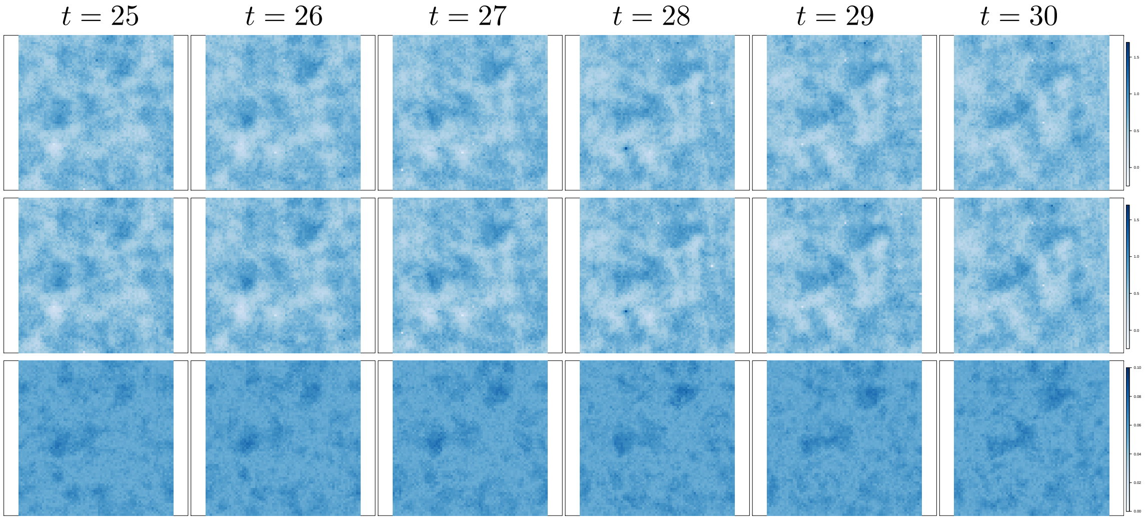
$t = 25$
$t = 26$
$t = 27$
$t = 28$
$t = 29$
$t = 30$

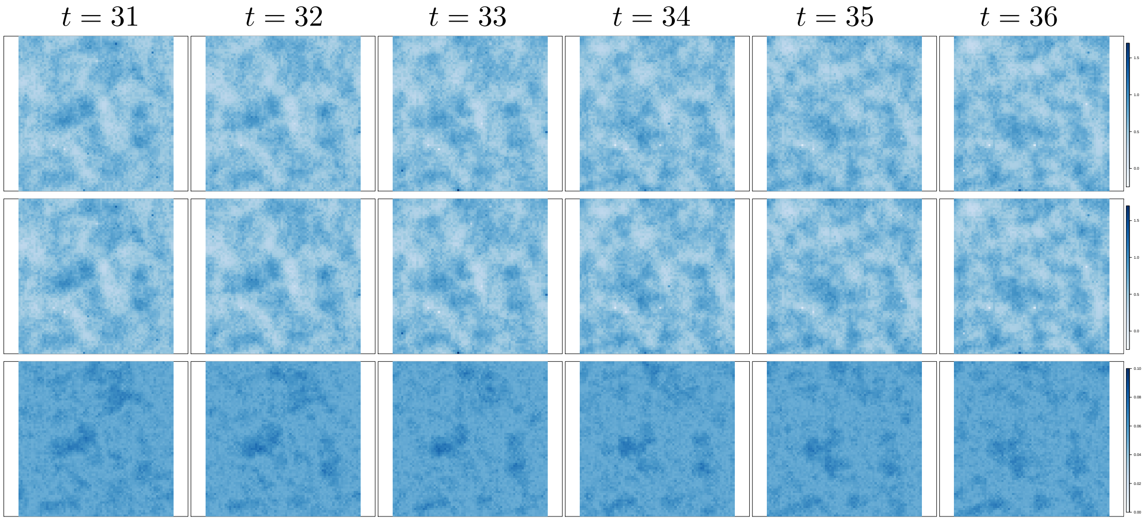
$t = 31$
$t = 32$
$t = 33$
$t = 34$
$t = 35$
$t = 36$

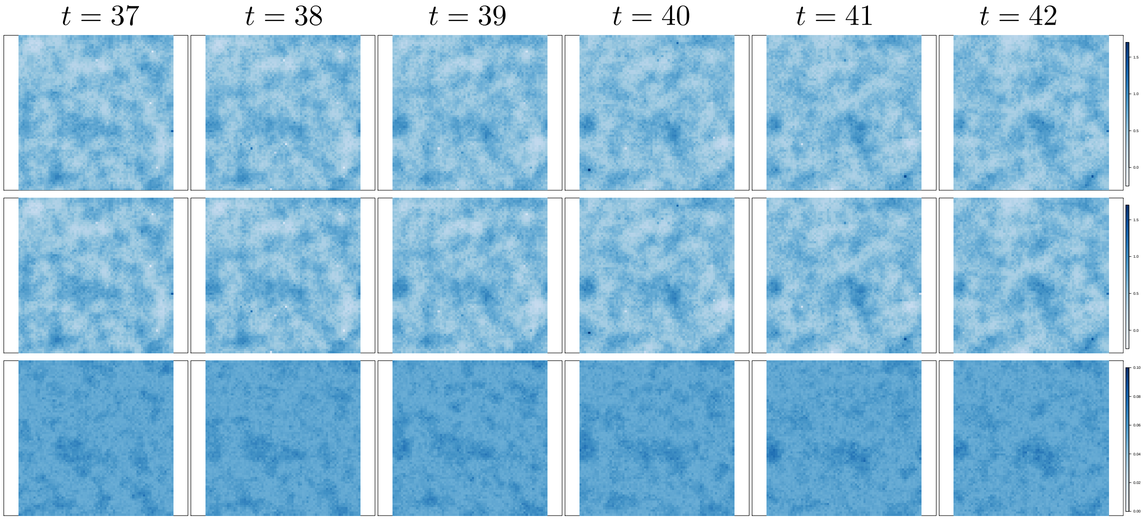
$t = 37$
$t = 38$
$t = 39$
$t = 40$
$t = 41$
$t = 42$

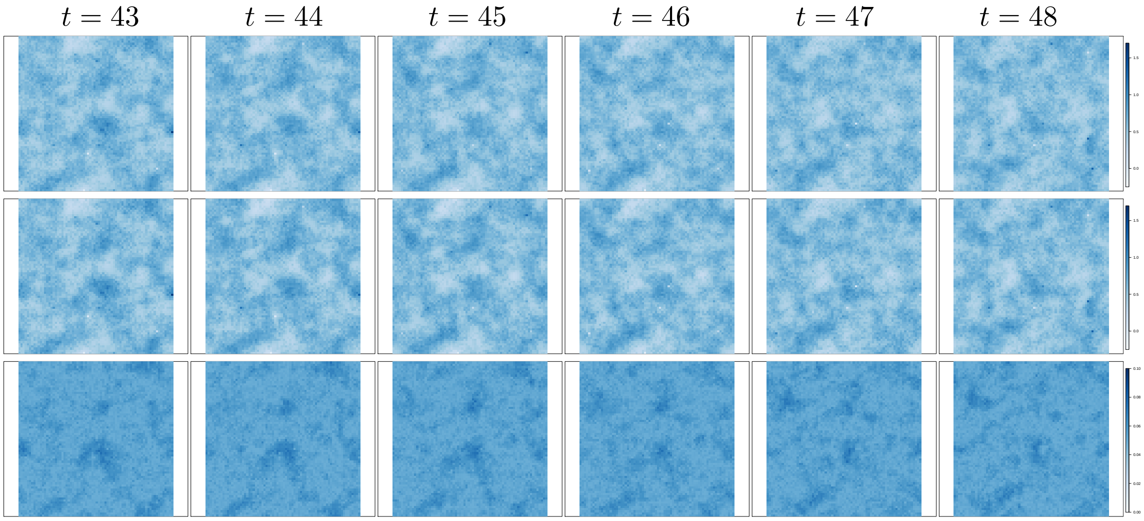
$t = 43$
$t = 44$
$t = 45$
$t = 46$
$t = 47$
$t = 48$

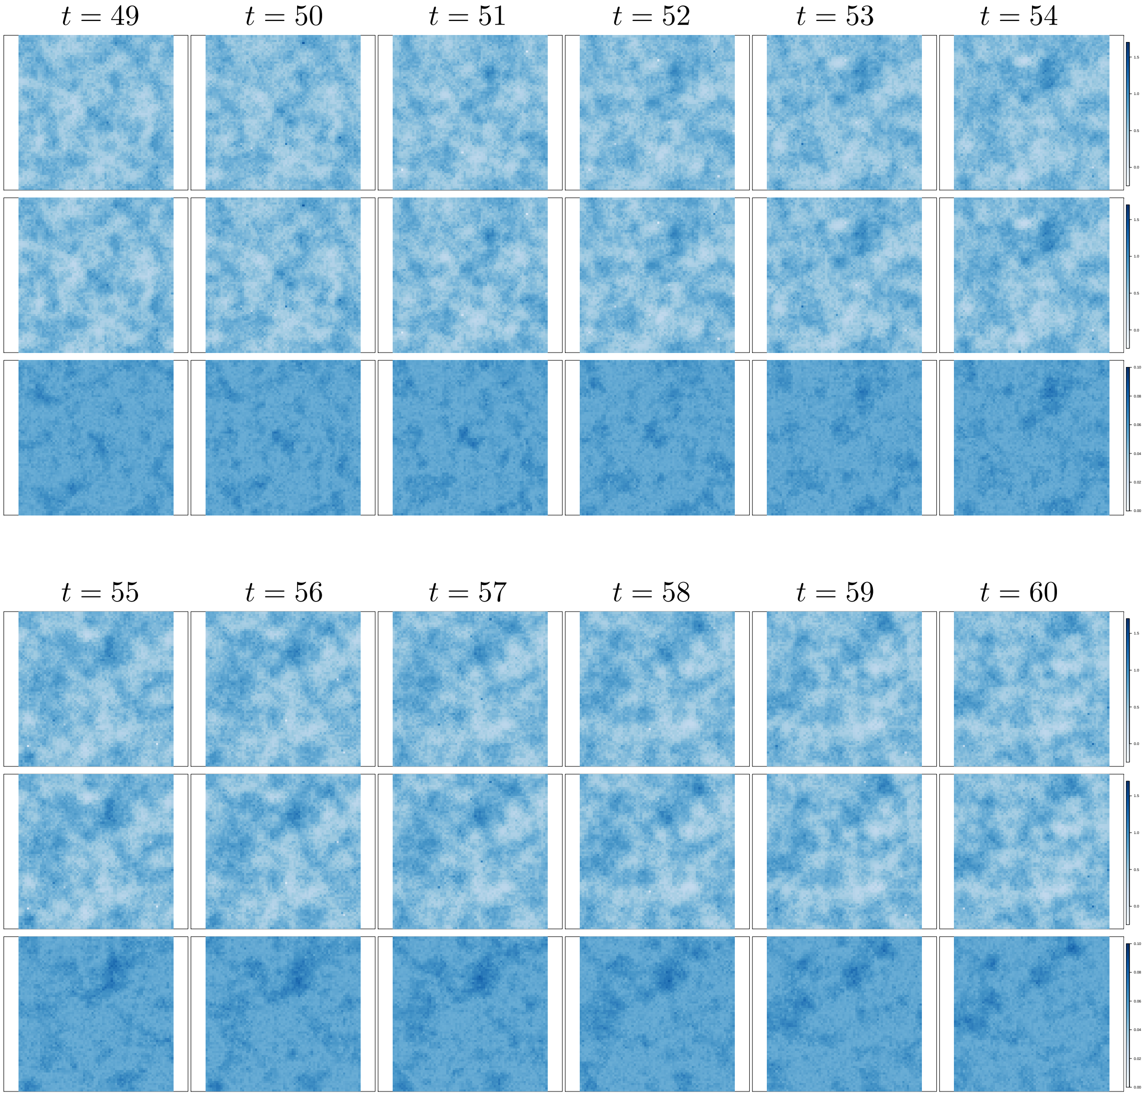
$t = 49$
$t = 50$
$t = 51$
$t = 52$
$t = 53$
$t = 54$
$t = 55$
$t = 56$
$t = 57$
$t = 58$
$t = 59$
$t = 60$

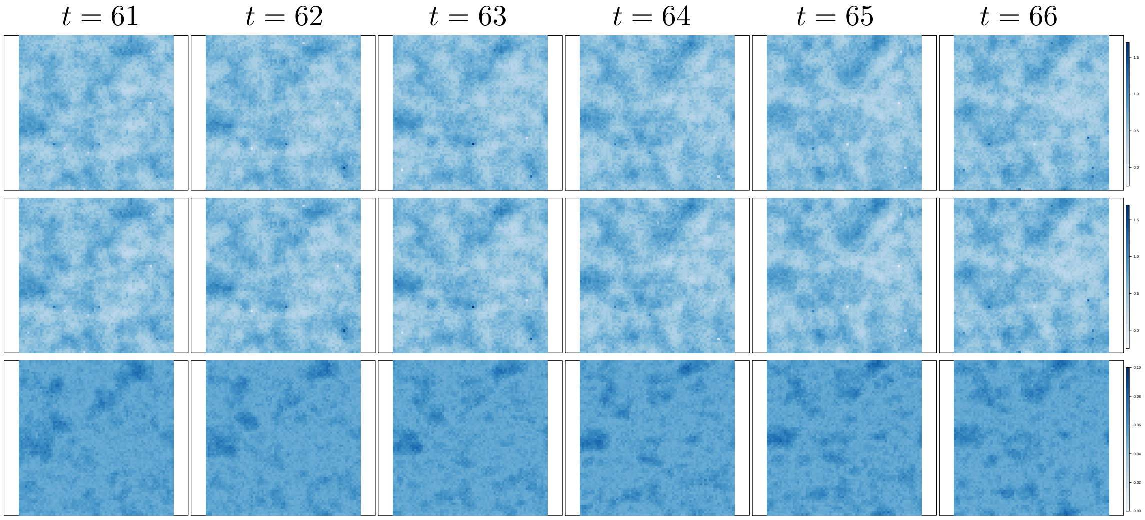
$t = 61$
$t = 62$
$t = 63$
$t = 64$
$t = 65$
$t = 66$

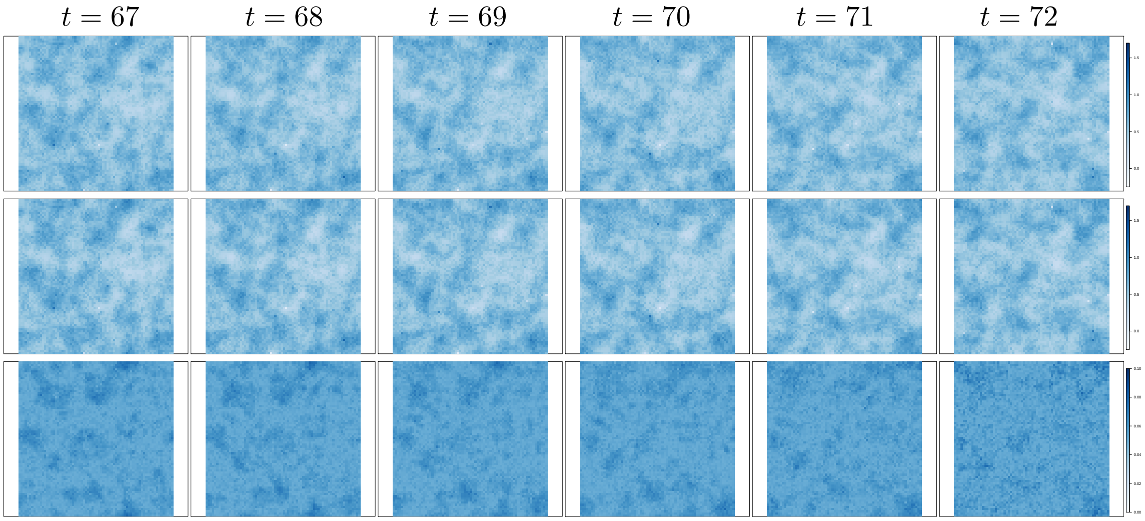
$t = 67$
$t = 68$
$t = 69$
$t = 70$
$t = 71$
$t = 72$

# 4 Real data images

This section contains figures akin to Figure 2 in the paper for all observation times $t = 1, \ldots, 72$. More specifically, in each collection of figures below, the top row shows image plots of the (transformed) radar observations $\tilde{\boldsymbol{y}}_t^{\mathrm{r}}$, the marginal posterior means ($\mathrm{E}(\theta_{ti}|\mathcal{D})$, $i = 1, \ldots, N$) of the precipitation field of interest are shown in the second row and the corresponding (marginal) standard deviations ($\mathrm{SD}(\theta_{ti}|\mathcal{D})$, $i = 1, \ldots, N$) are shown in the third row. The fourth row shows the posterior probability $\Pr(\theta_{ti} > 0|\mathcal{D})$ and the final row contains boxplots of the marginal posterior distributions of the precipitation field at the rain gauge locations, $\pi(\theta_{t,\ell_g}|\mathcal{D})$ for $g = 1, \ldots, 15$; crosses show the (transformed) gauge observations $\tilde{\boldsymbol{y}}_t^{\mathrm{g}}$.

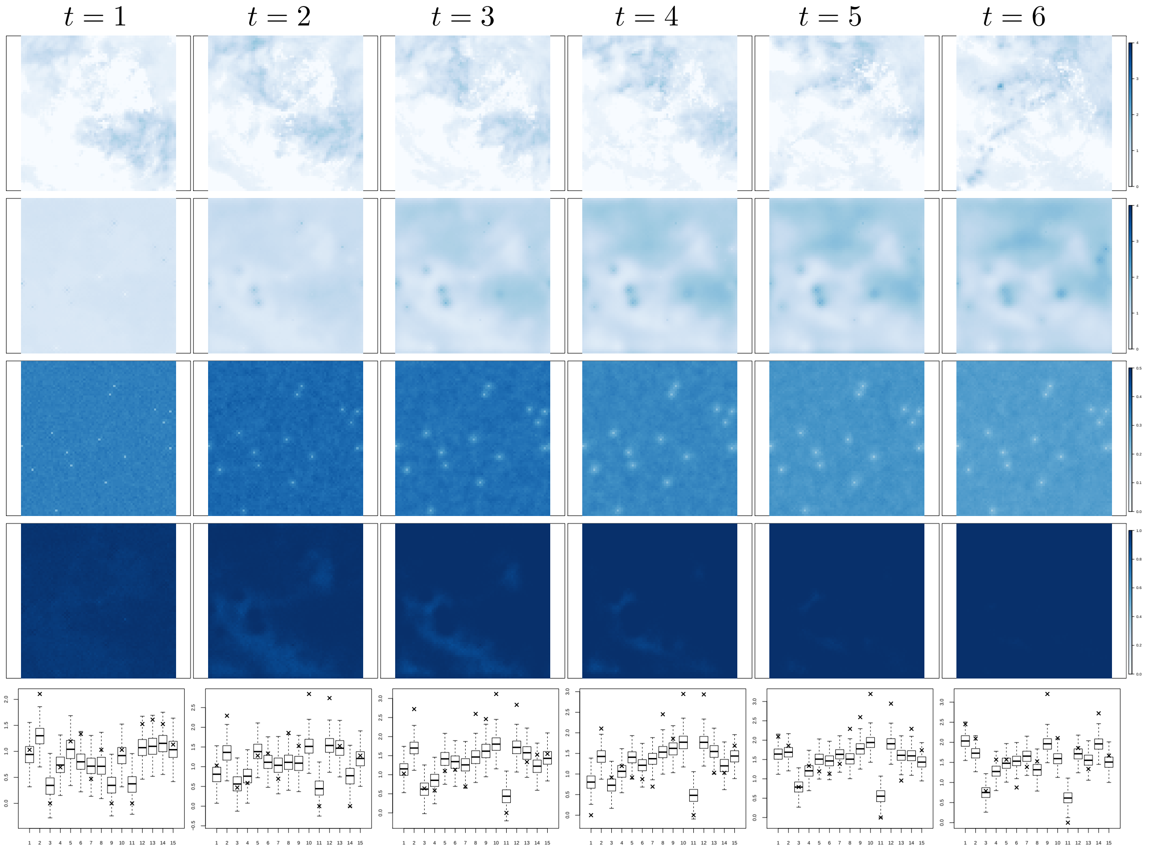

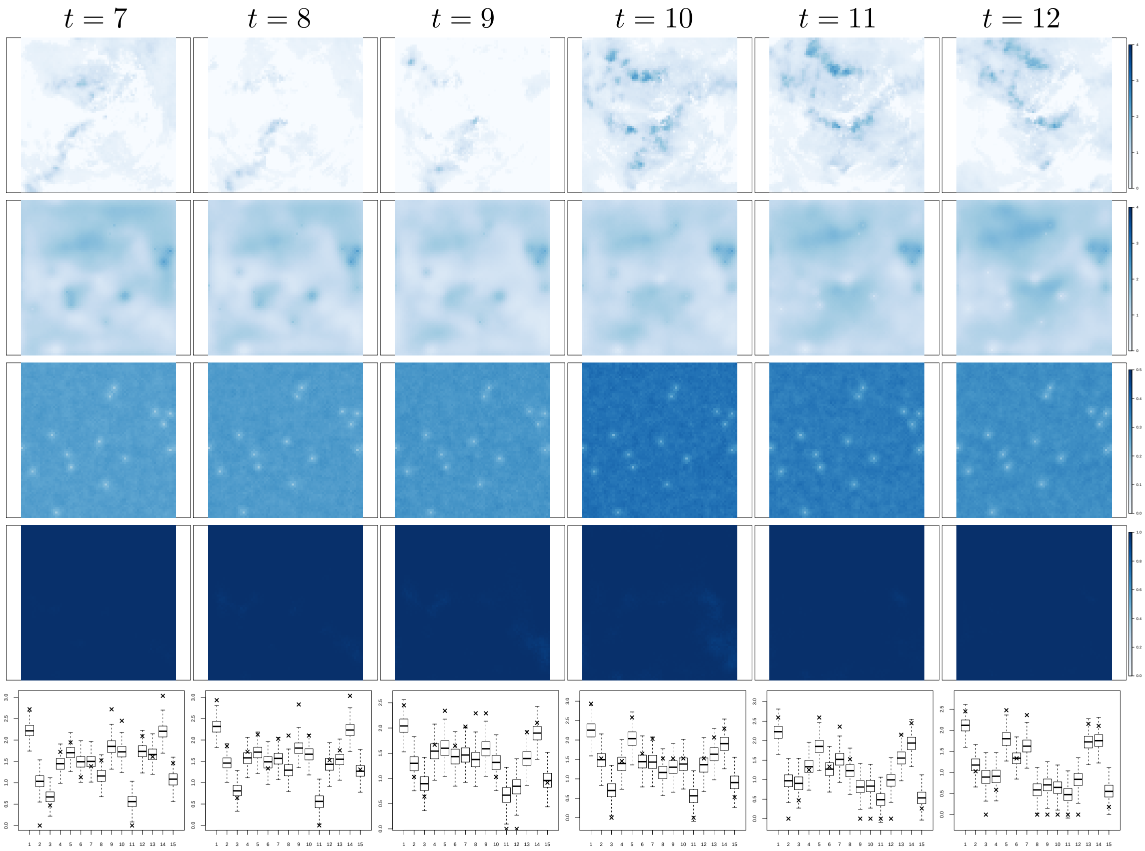
$t = 7$
$t = 8$
$t = 9$
$t = 10$
$t = 11$
$t = 12$

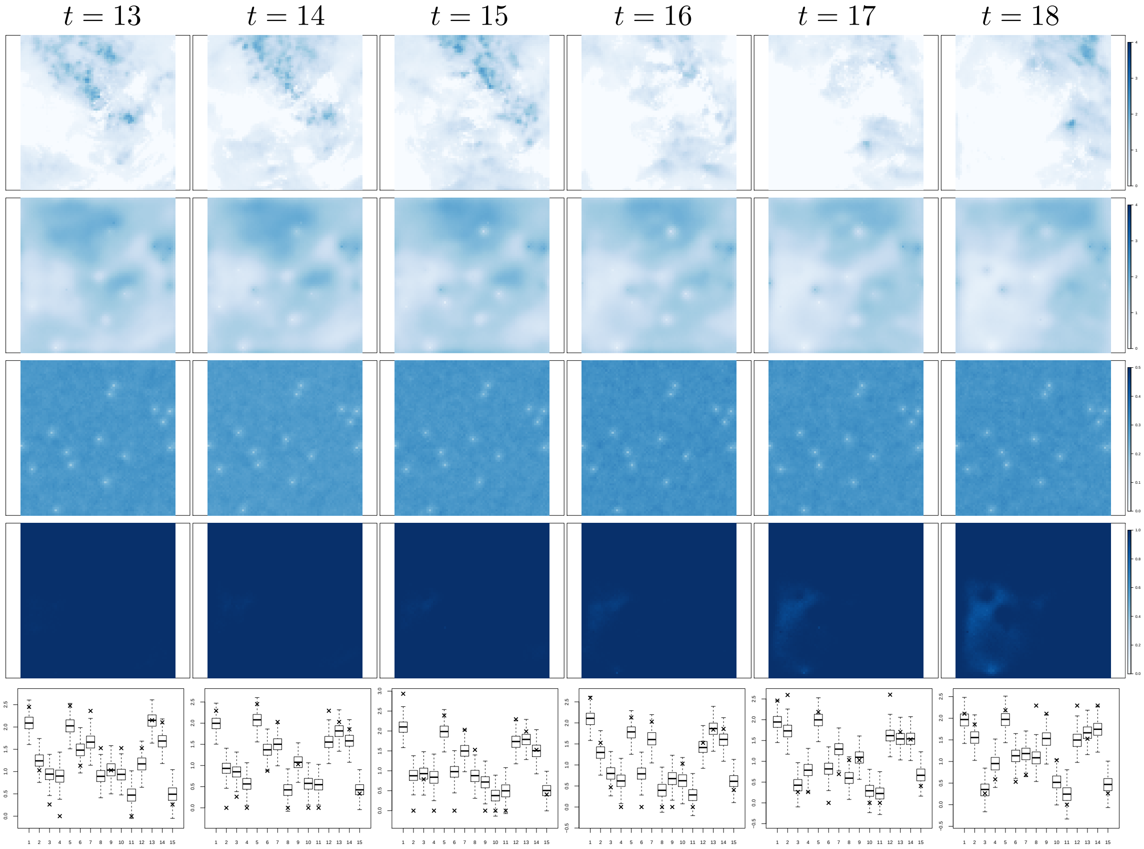
$t = 13$
$t = 14$
$t = 15$
$t = 16$
$t = 17$
$t = 18$

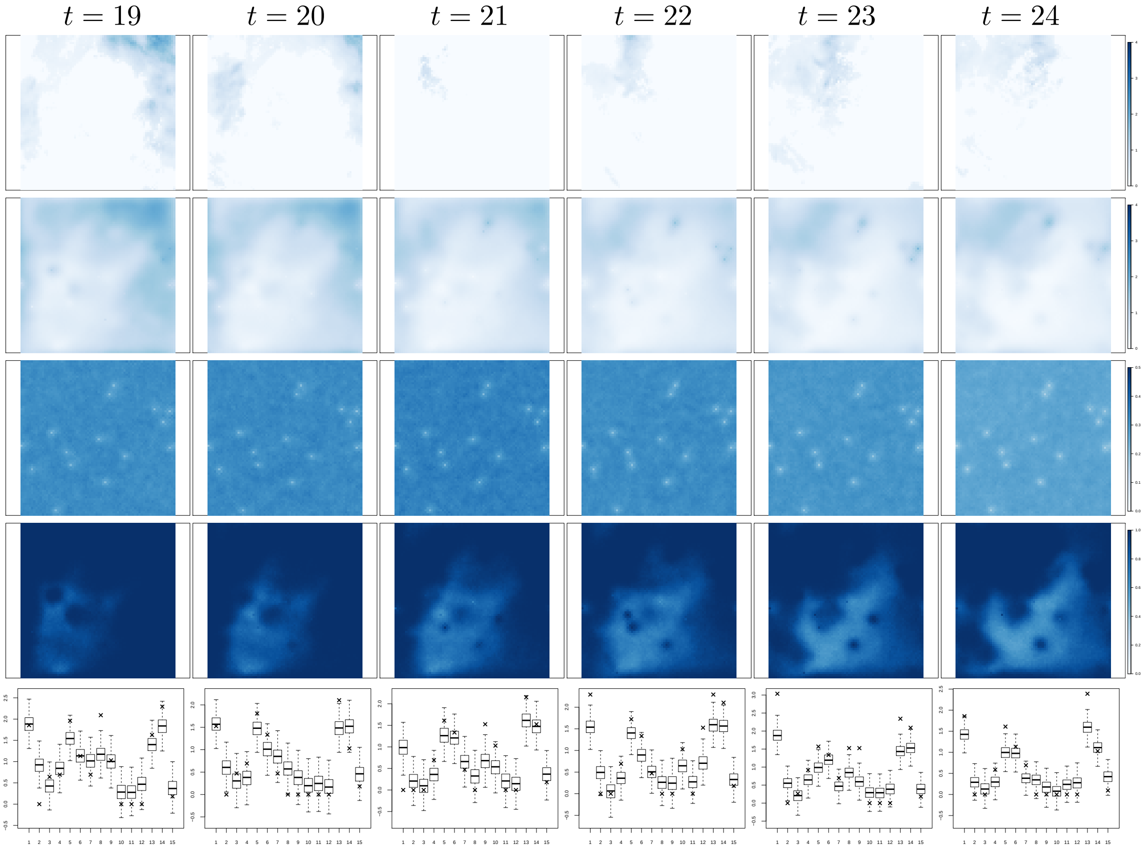
$t = 19$
$t = 20$
$t = 21$
$t = 22$
$t = 23$
$t = 24$

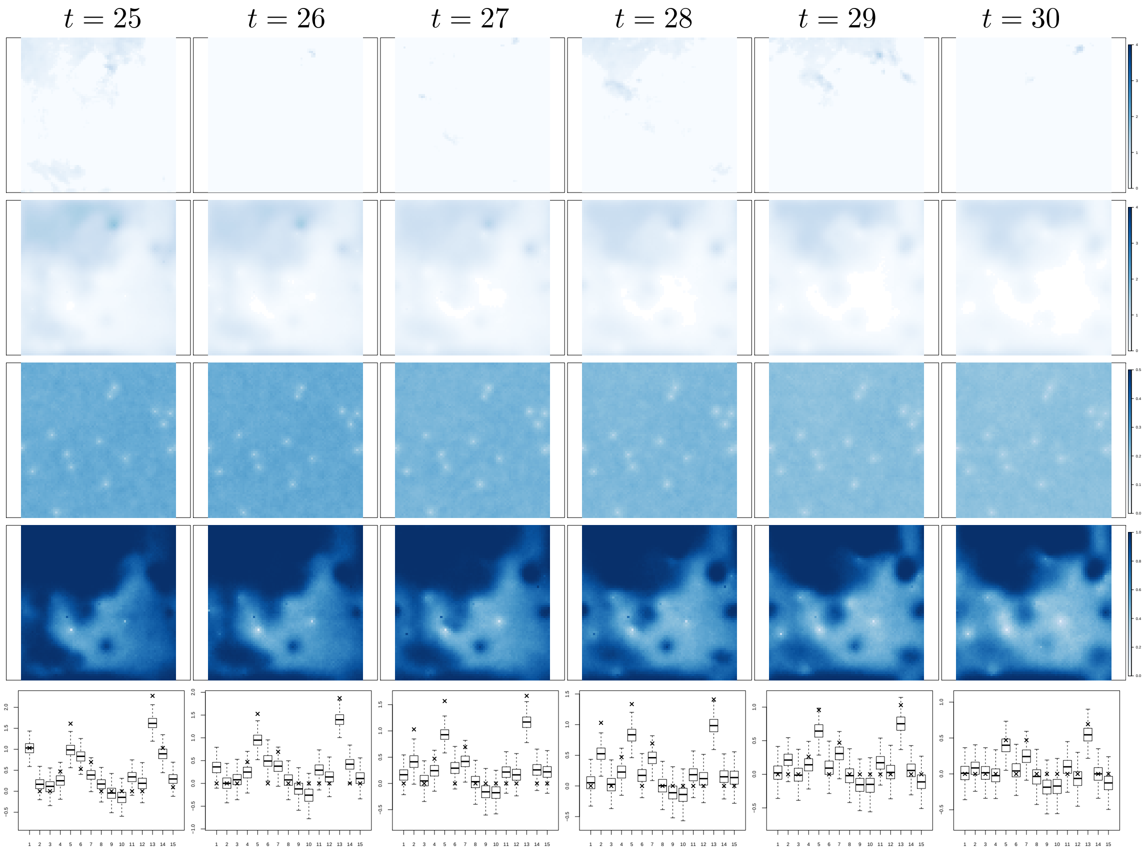

$t = 25$
$t = 26$
$t = 27$
$t = 28$
$t = 29$
$t = 30$

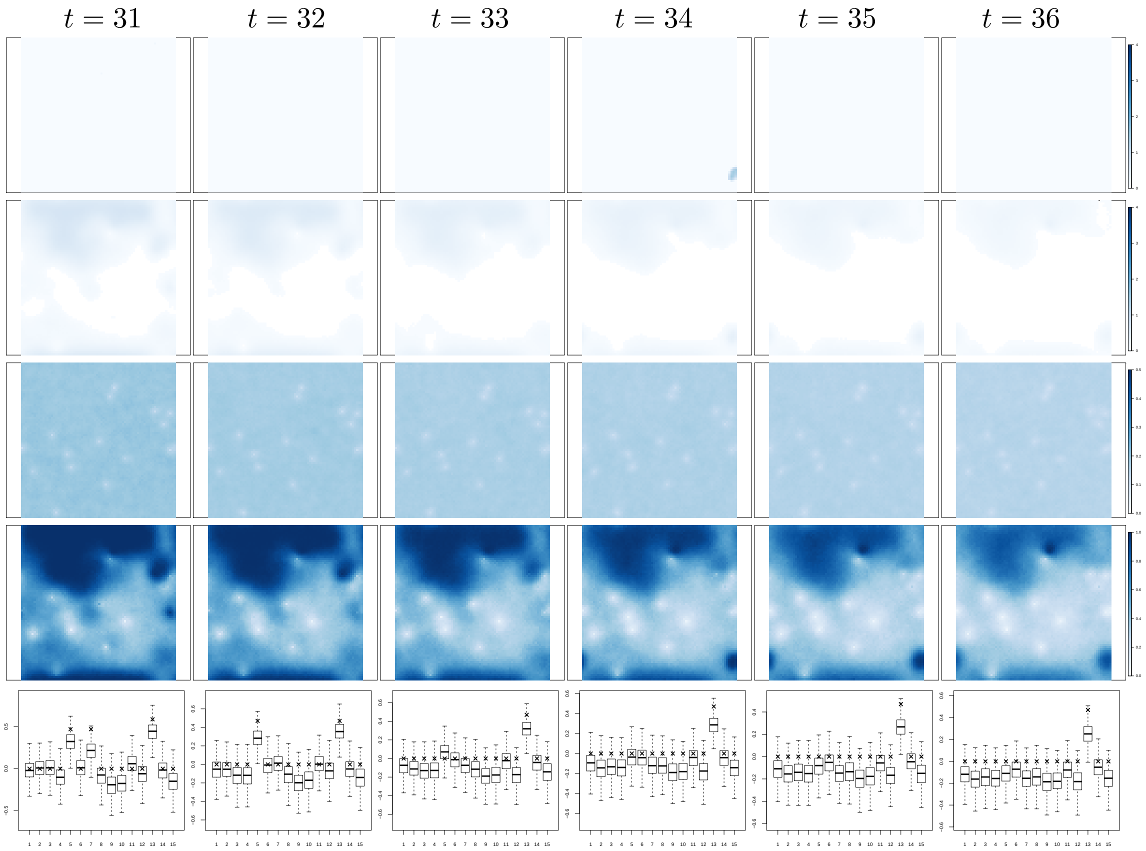
$t = 31$
$t = 32$
$t = 33$
$t = 34$
$t = 35$
$t = 36$

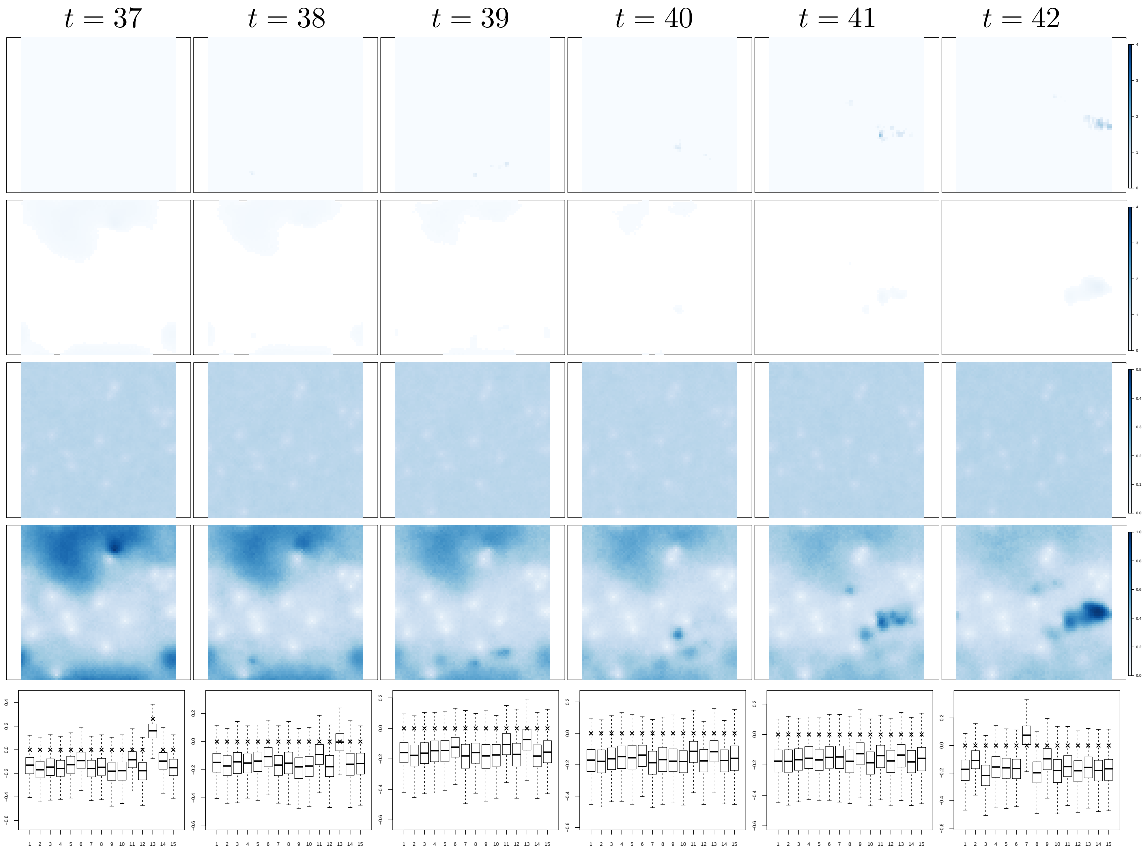

$t = 37$
$t = 38$
$t = 39$
$t = 40$
$t = 41$
$t = 42$

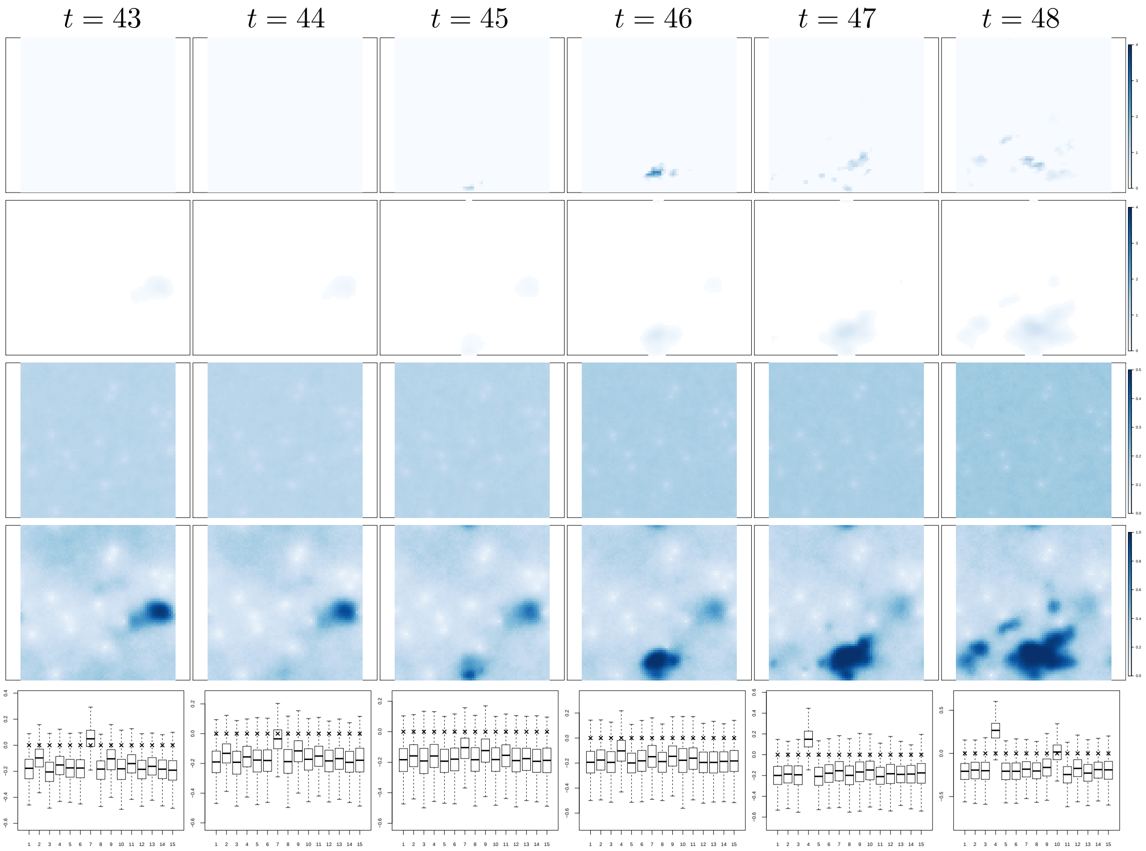
t = 43
t = 44
t = 45
t = 46
t = 47
t = 48

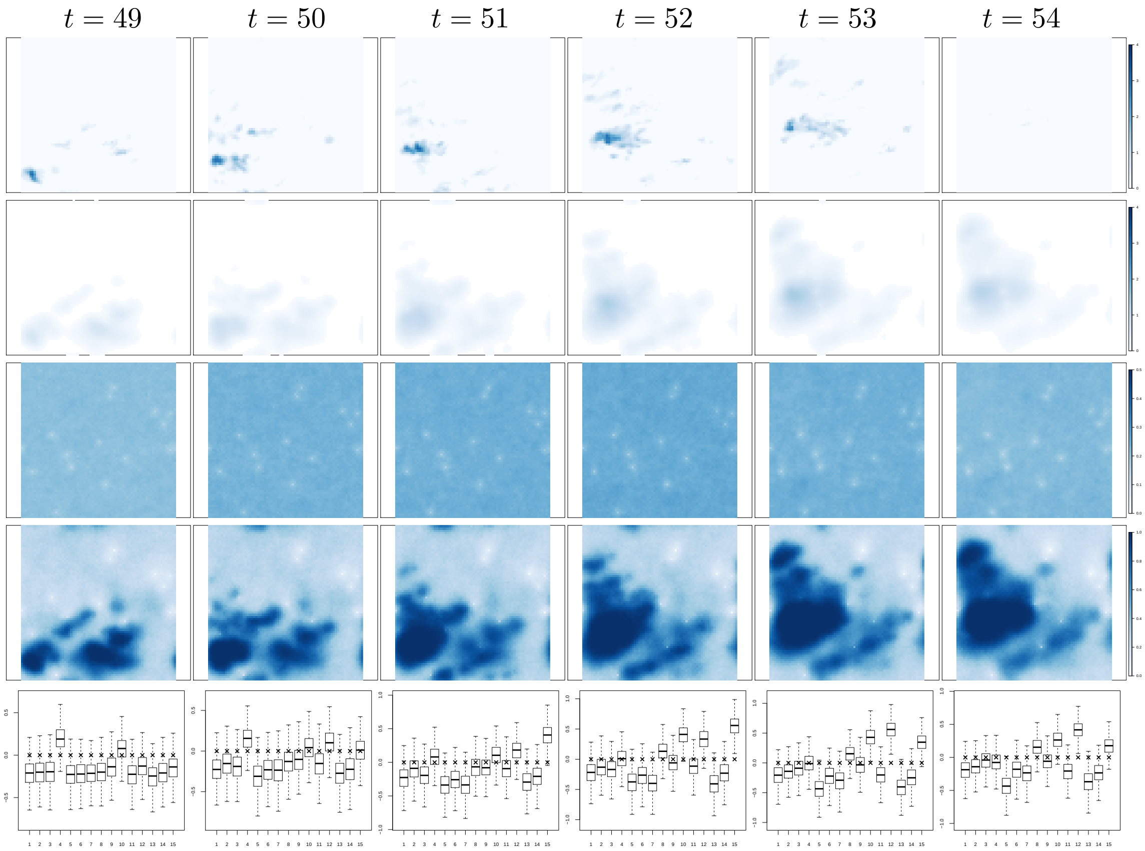
$t = 49$
$t = 50$
$t = 51$
$t = 52$
$t = 53$
$t = 54$

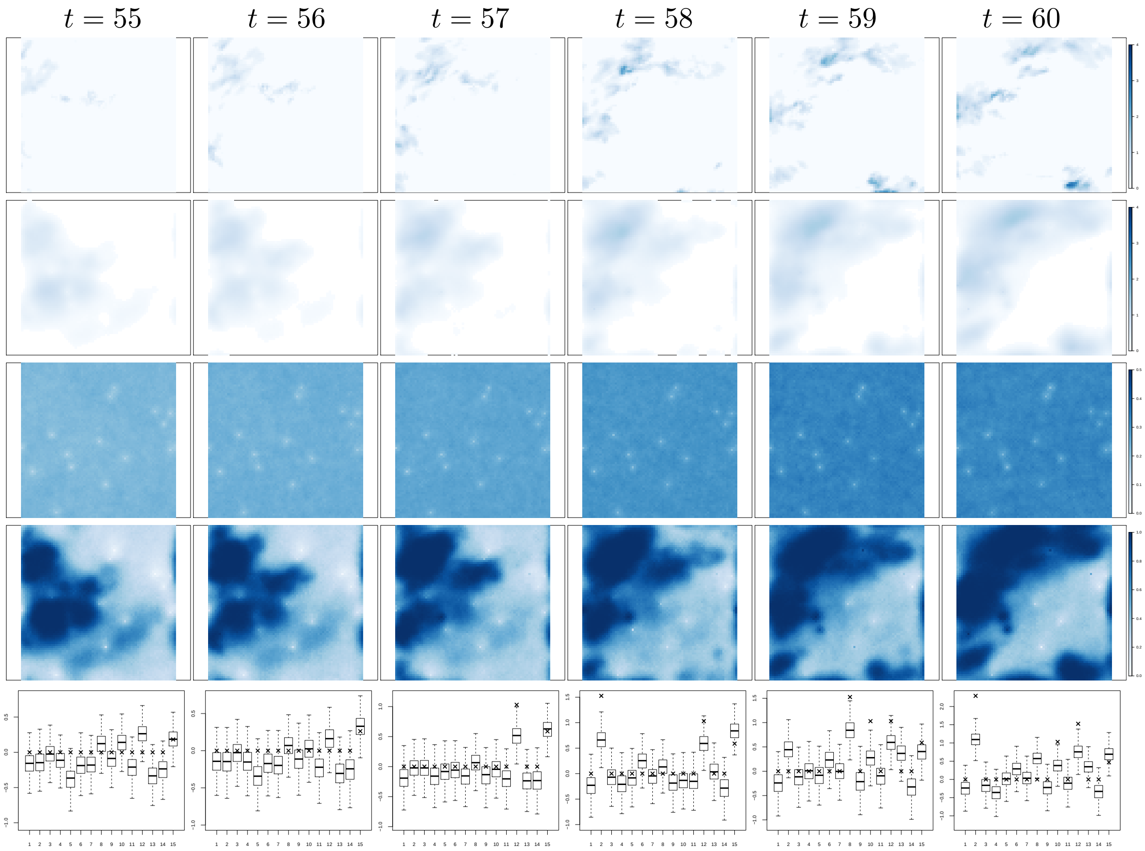
$t = 55$
$t = 56$
$t = 57$
$t = 58$
$t = 59$
$t = 60$

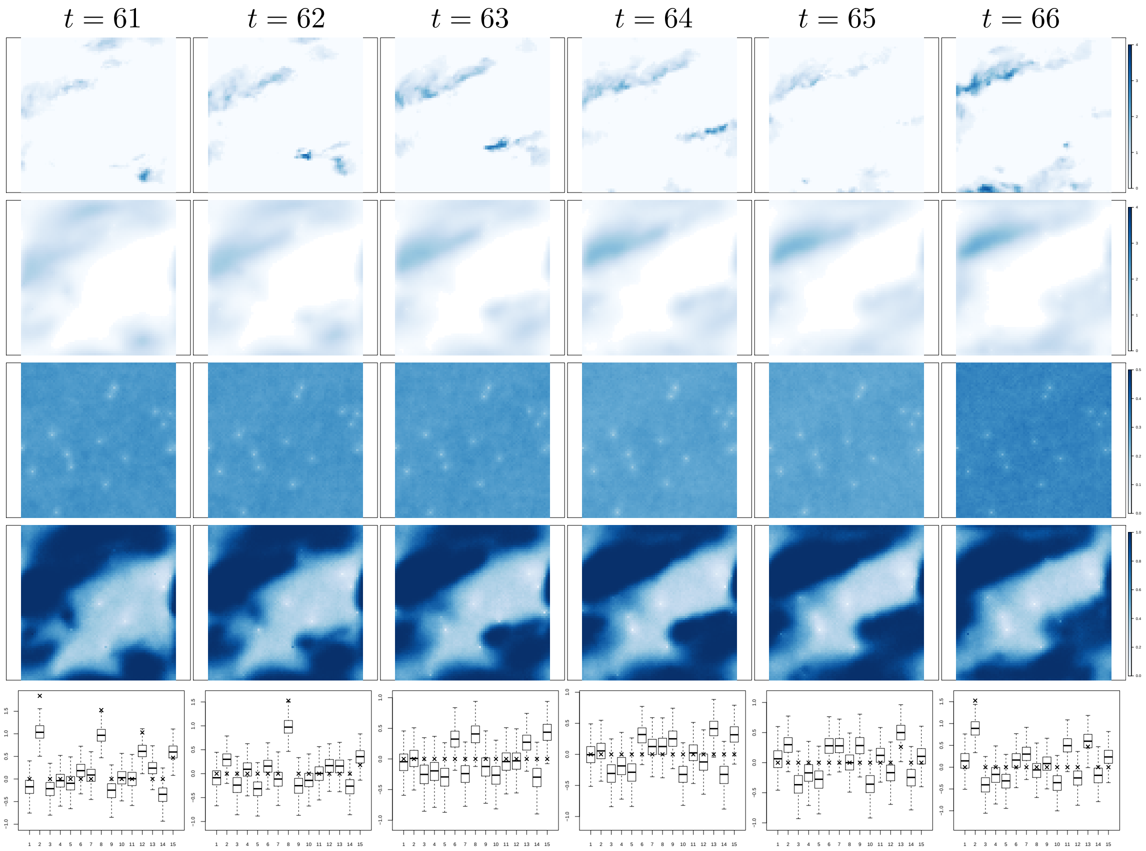
$t = 61$
$t = 62$
$t = 63$
$t = 64$
$t = 65$
$t = 66$

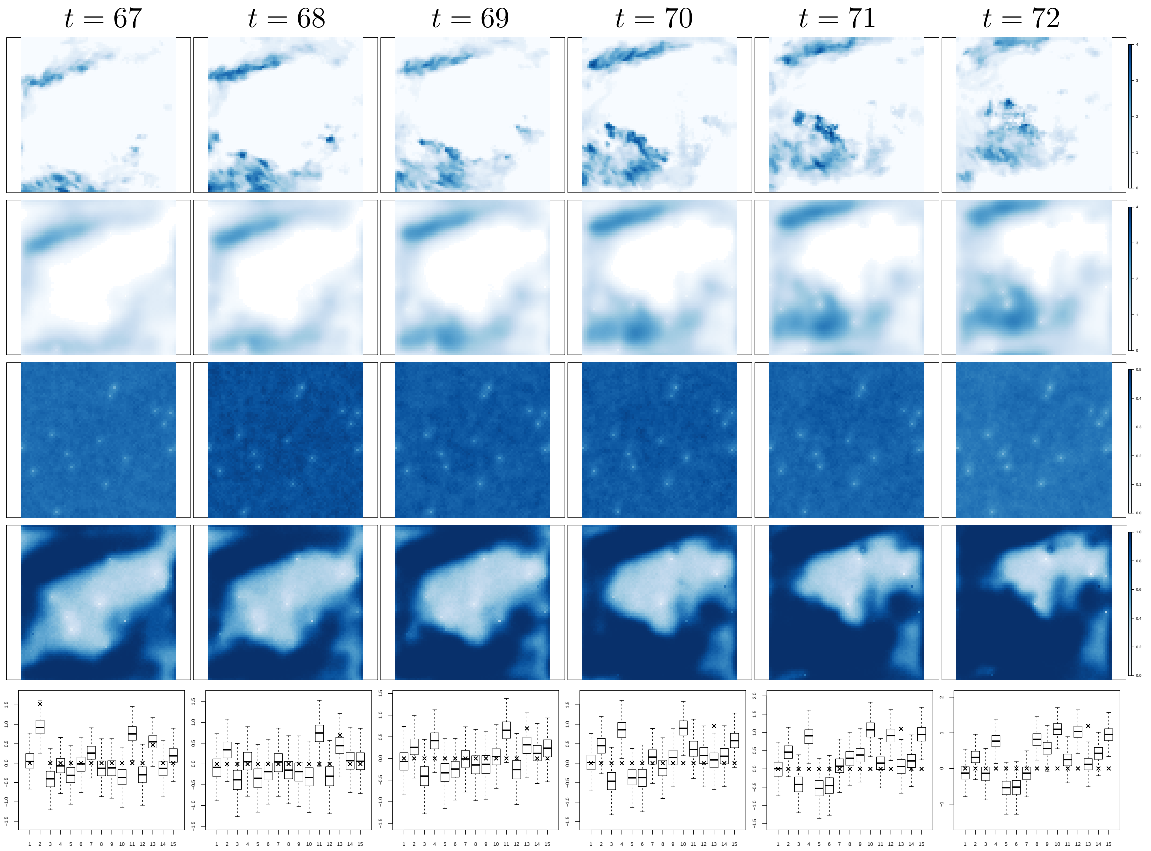

# References


Anderson, J. L. and S. L. Anderson (1999). A Monte Carlo implementation of the nonlinear filtering problem to produce ensemble assimilations and forecasts. *Monthly Weather Review 127*(12), 2741–2758.

Evensen, G. (2003). The ensemble Kalman filter: Theoretical formulation and practical implementation. *Ocean dynamics 53*(4), 343–367.

Houtekamer, P. L. and H. L. Mitchell (2001). A sequential ensemble Kalman filter for atmospheric data assimilation. *Monthly Weather Review 129*(1), 123–137.
